# Supplementary material for: Multi-Camera Calibration Free BEV Representation for 3D Object Detection
Source: arXiv:2210.17252 source file (2022-10-31)
Supplement: Supplementary file 1 [file Fig-supp-vis.tex]

\begin{figure}[h]
     \centering
     \begin{subfigure}[b]{\textwidth}
         \centering
         \makebox[\textwidth][c]{\includegraphics[width=1.2\textwidth]{images/1.pdf}}
         \label{fig:1}
     \end{subfigure}
     \vfill
     \begin{subfigure}[b]{\textwidth}
         \centering
         \makebox[\textwidth][c]{\includegraphics[width=1.2\textwidth]{images/2.pdf}}
         \label{fig:2}
     \end{subfigure}
     \caption{Visualizations (Part I): Given multi-camera images, our method dedicates to perform 3D object detection and BEV semantic segmentation.}
     \label{fig:supp_vis_1}
\end{figure}
\begin{figure}[htbp]
     \centering
     \begin{subfigure}[b]{\textwidth}
         \centering
         \makebox[\textwidth][c]{\includegraphics[width=1.2\textwidth]{images/3.pdf}}
         \label{fig:3}
     \end{subfigure}
     \vfill
     \begin{subfigure}[b]{\textwidth}
         \centering
         \makebox[\textwidth][c]{\includegraphics[width=1.2\textwidth]{images/4.pdf}}
         \label{fig:4}
     \end{subfigure}
      \caption{Visualizations (Part II): Given multi-camera images, our method dedicates to perform 3D object detection and BEV semantic segmentation.}
     \label{fig:supp_vis_2}
\end{figure}
